# Supplementary material for: HOOD: Hierarchical Graphs for Generalized Modelling of Clothing Dynamics
Source: arXiv:2212.07242 source file (2023-06-16)
Supplement: Supplementary file 1 [file 101_experiments_suppmat.tex]

\section{Experiment details}

We trained our final model for 150000 training iterations which took around 26 hours on NVIDIA Quadro RTX 6000 GPU.

Below we provide some additional information concerning the experiments from the main paper.

\subsection{Comparison to state-of-the-art}

Since we do not learn for the physically simulated data as~\cite{Santesteban_2021_CVPR} does and use slightly different objective function form SNUG~\cite{santesteban2022snug} (See Sec.~\ref{sec:supervision}), it is difficult to quantitatively our method to them. However, we can compute the size and the number of body-garment penetrations by our method and the baselines. We provide these values in Table~\ref{table:coll}

\begin{table}[ht]
    \centering
    \resizebox{1\linewidth}{!}{
    \begin{tabular}{c|c|cccccc}
                                  &   garments   & $\mathcal{L}_{collision}$ & \% penetrating vertices    \\ \hline
     SNUG~\cite{santesteban2022snug} & t-shirt, long sleeve top,& 1.81e-8 &  1.26e-5 \\
     Ours                              & tank top, pants, shorts   &  \textbf{2.69e-10} & \textbf{2.55e-6} \\ \hline
     SSCH\cite{Santesteban_2021_CVPR} & \multirow{2}{*}{t-shirt, dress} &   5.3e-8 &   1.23e-5 \\
     Ours                              &   &     \textbf{1.22e-9} &  \textbf{2.38e-7}                    
    \end{tabular}}
    \caption{Our method generates fewer garment-body penetrations compared to state-of-the-art methods in terms of both average penetration size and percentage of garment vertices penetrating the body. The numbers were averaged over the whole validation set.}
    \label{table:coll}
\end{table}

\subsection{Architecture analysis}

In addition to Table 1 in the main paper, we provide detailed metrics averaged across the whole validation set for our final model \textit{Ours} and two baseline architectures \textit{Fine15} and $Fine48$ in Table~\ref{table:coarse_metrics}.

Different architectures with different sets of fine and coarse message-passing steps may result in models with different inference speeds, propagation radii and levels of fine details. We demonstrate the qualitative differences between different architectures in the supplementary video \textit{additional\_videos/architectures.mp4}.

\begin{table*}[]
    \centering
    \resizebox{0.8\linewidth}{!}{
\begin{tabular}{c|c|c|ccccccc}
                        & garments  & average speed, fps                   & $\mathcal{L}_{stretching}$            & $\mathcal{L}_{bending}$          & $\mathcal{L}_{inertia}$   &  $\mathcal{L}_{gravity}$  &  $\mathcal{L}_{collision}$   &  $\mathcal{L}_{friction}$     \\ \hline
\textit{Fine15} & \multirow{3}{*}{only dress} & 6.65 &  3.73e-3          & 3.28e-5         & 1.26e-5 & \textbf{2.24e-3} & 5.74e-9 & 5.68e-6      \\
\textit{Fine48} &                             & 2.45 & \textbf{3.95e-4} & \textbf{2.71e-5} & 9.28e-6  & 2.3e-3 & 1.96e-9 & 5.44e-6 \\
\textit{Ours\_full}     &                     & \textbf{7.27} &  5.22e-4          & 3.32e-5       &   \textbf{8.48e-6} & 2.3e-3 & \textbf{1.7e-9} & \textbf{4.83e-6} \\ \hline
\textit{Fine15} & \multirow{3}{*}{all}      & 13.1  & 2.2e-3         & 1.51e-5          & 8.06e-6  & \textbf{1.41e-3} & 1.5e-9 & 2.92e-6  \\
\textit{Fine48} &                          & 4.99  & \textbf{2.68e-4} & \textbf{1.36e-5}             &  7.2e-6 & 1.42e-3 & 5.54e-10 & 2.77e-6    \\
\textit{Ours\_full}     &                  &  \textbf{13.6} & 3.59e-4          & 1.53e-5 & \textbf{6.76e-6} & 1.43e-3 & \textbf{4.48e-10} & \textbf{2.55e-6}
\end{tabular}
    }
    \caption{Comparison of our final model to two ablations in terms of physical objectives and inference speed. We provide the metrics for the largest garment in the training set (\textit{dress}, 12K vertices) separately.}
    \label{table:coarse_metrics}
\end{table*}

\begin{figure}[t]
  \centering
  \includegraphics[width=0.9\linewidth]{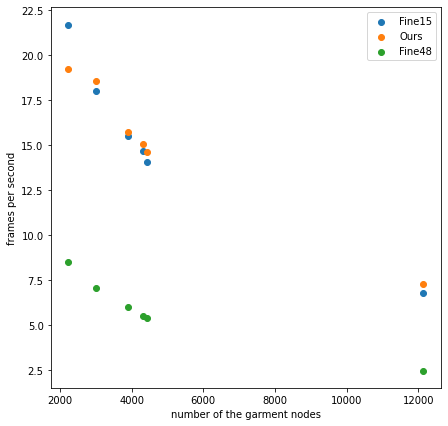}

  \caption{Inference speed in frames per second for our final model and two baseline architectures. Each point corresponds to one of the training garments. The speed was measured using NVIDIA GeForce RTX 3060 GPU}
  \label{fig:speed}
\end{figure}
